# Supplementary material for: Pushing the Boundaries of Tractable Multiperspective Reasoning: A Deduction Calculus for Standpoint EL+
Source: arXiv:2304.14323 source file (2023-05-11)
Supplement: Supplementary file 1 [file appendix.tex]

\section{Proofs for \Cref{sec:syntax-semantics}}

\input{sections/normal-form.tex}

\section{Proofs for \Cref{sec:tableau}}

We structure the proofs for \Cref{sec:tableau} in two subsections. In \Cref{sec:app-termination}, we provide the proof of  \Cref{theorem:termination} \emph{(Termination)} and some intermediary lemmas and their proofs. In \Cref{sec:app-soundness-completeness}, we provide the full proofs of \Cref{theorem:soundness} \emph{(Soundness)} and \Cref{theorem:completeness} \emph{(Completeness)}, as well as some intermediary lemmas and their proofs.

\subsection{Termination}\label{sec:app-termination}

For convenience of presentation, let $\stvar{S}{\st} \eqdef  \{v \mid (v\col \st)\in S\}$ denote the set of $\st$-variables in a constraint system $S$, and let $\stvar{\qelem}{\st}$ be the sortcut for $\stvar{\consis{\qelem}}{\st}$.

\begin{lemma}\label{lemma:preceq-axioms-everywhere}
    Let $S$ be a constraint system for $\kb$ produced by the algorithm. Then $(\st\preceq\sp)\in\kb$ iff there is some $x$ such that $(x\col \st\preceq\sp)\in S$.
\end{lemma}

\begin{proof}
    ($\Rightarrow$) From the definition of a constraint system for $\kb$, for all $(\st\preceq\sp)\in\kb$ we have $(v_{*}\col \st\preceq\sp)\in S$. ($\Leftarrow$) It is easy to see from the tableau rules that $(x\col \st\preceq\sp)$ can only be introduced during the creation of $S$ or by copying a preexisting $(x'\col \st\preceq\sp)$ constraint in $S$. If $S$ is created during the initialisation of the algorithm, then $(x\col \st\preceq\sp)\in S$ because $(\st\preceq\sp)\in\kb$. Similarly, if $S$ is created by an $\mathbf{R}_{\exists}$ application, then  $(x\col \st\preceq\sp)\in\consis{\qelem_{\top}}$ and hence also $(\st\preceq\sp)\in\kb$.
\end{proof}

\def\initialcsll{S_{L}^{\kb}}

\begin{lemma}\label{lemma:same-standpoints}
    Let $S$ and $S'$ be locally complete constraint systems for $\kb$ produced by the algorithm.
    The set of `standpoint signatures' in $S$ and $S'$ is the same $\{ \stlabel{S}{v} \mid v \in\stvar{S}{*}\}=\{ \stlabel{S'}{v} \mid v \in\stvar{S'}{*}\}$ and its size is smaller or equal to the number of standpoints in $\kb$, i.e. $\card{\{ \stlabel{S}{v} \mid v \in\stvar{S}{*}\}} \leq \card{\SC}$.
\end{lemma}

\begin{proof}
    Let $\initialcsll$ be the constraint system obtained by exhaustively applying (only) the local labelling rules to $\initialcs$.
    It is clear that $\initialcsll$ has exactly $\card{\SC}$ variables and hence there are at most $\card{\SC}$ different standpoint signatures. We will prove the lemma by showing that for $S$ a constraint system for $\kb$ where no local rules are applicable, the set of standpoint labels in $S$ and $\initialcsll$ is the same.

    Upon observation of the tableau rules, we can see that for any variable $v$ in $S$ either
    \begin{description}
        \item{\bf Base Case:} $v$ is initialised with $\{v\col \st,v\col * \}\subseteq  S$.
        By the definition of $\initialcs$, there is a variable $v_{\st}$ in $\initialcs$ also initialised with $\{v_{\st}\col \st,v_{\st}\col * \}\subseteq\initialcs$. Then, from Lemma \ref{lemma:preceq-axioms-everywhere} it follows that for some $x$ in $S$ and $x'$ in $S'$, we have $(x\col \sp\preceq\st)\in S$ iff $(x'\col \sp\preceq\st)\in S'$ iff $(\sp\preceq\st)\in\kb$. Moreover, from the definition of a constraint system, if $(\sp\preceq\st)\in\kb$ then $(v_{*}\col \sp\preceq\st)$ in both $S$ and $S'$
        Thus, by the premise, the tableau rules and the former observations, if $(v\col \s{n})\in S$ and $\s{n}\notin\{\st, *\}$ then there is a chain $\{(v_{*}\col \s{0}\preceq\s{1}),\dots,(v_{*}\col \s{n-1}\preceq\s{n})\}\subseteq S$ with $\s{0}\in\{\st, *\}$ such that the respective $\mathbf{R}_{\preceq}$ rule applications introduced $(v\col \s{n})$ in $S$. Also, $\{(v_{*}\col \s{0}\preceq\s{1}),\dots,(v_{*}\col \s{n-1}\preceq\s{n})\}\subseteq S'$ such that the respective $\mathbf{R}_{\preceq}$ rule applications introduced $(v'\col \s{n})\in S'$. Consequently, we obtain $\stlabel{S}{v}=\stlabel{\initialcsll}{v_{\st}}$ as desired.
        \item{\bf Inductive Step:} $v$ is initialised with $\{v\col\st \mid (v'\col \st)\!\in\! S', \st\!\in\!\SC \}$ for some $v'$ in $S'$. By induction, we know that for $v'$ in $S'$ there is some $x$ in $\initialcs$ such that $\stlabel{S'}{v'}=\stlabel{\initialcsll}{x}$. By Lemma \ref{lemma:preceq-axioms-everywhere}, if $(x\col \st\preceq\sp)\in S$ for some $x$ in $S$ then $(\st\preceq\sp)\in\kb$ and then also $(x'\col \st\preceq\sp)\in S'$ for some variable $x'$ in $S'$. Thus, if $(v\col \sp)\in S$ then also $(v'\col \sp)\in S'$, and therefore  $\stlabel{S}{v}=\stlabel{S'}{v'}$. Consequently, $\stlabel{S}{v}=\stlabel{\initialcsll}{x}$ as desired.
    \end{description}
\end{proof}

\begin{lemma}\label{lemma:num-elements-cs}
    Let $\mathbf{CG}$ be a completion graph for $\kb$ constructed by the algorithm. The number of elements in $\mathbf{CG}$ is bounded by $3\size{\kb}^2$.
\end{lemma}

\begin{proof}
    Let us first consider the number of elements in $\mathbf{CG}$ in its initialisation and then the number of new elements that can be produced by global rule applications. It is easy to see that during initialisation, we will produce exactly $1+\card{\objC}$ elements and $1+\card{\objC}\leq \size{\kb}$ (there is at least one formula in $\kb$). The applicability of the global generating rules depends on the preexistence of element labels of the form $(C,s,x)\in L$ that are different to the current node. Since global rules are only applicable to locally complete constraint systems (by the order imposed by the algorithm) and by Lemma \ref{lemma:same-standpoints} we know that there are at most $\card{\SC}$ different standpoint signatures in $\mathbf{CG}$ if it is locally consistent, then the rule $\mathbf{R}_{\exists}$ can produce at most $2\card{\SC}\times\card{\CC}\leq 2\size{\kb}^2$ different elements before no rules are applicable in $\mathbf{CG}$.
\end{proof}

\begin{lemma}\label{lemma:num-constraints-per-element}
    Let $\mathbf{CG}$ be a completion graph for $\kb$ constructed by the algorithm and $\qelem$ be an element in $\mathbf{CG}$. The number of variables in $\consis{\qelem}$ is bounded by $2\size{\kb}^2$ and the number of constraints in $\consis{\qelem}$ by $2\size{\kb}^3$.
\end{lemma}

\begin{proof}
    Let us determine an upper bound for the number of distinct variables
    per element. First, an element produced during the initialisation of the tableau $\qelem_i\in\{\qelem_{\top}\}\cup\{\qelem_a\mid a\in\objC\}$ (its label, to be more precise) contains exactly $|\SC|$ distinct variables at the moment of its generation.% Since new marked variables are never produced, each element will always have at most $|\SC|$ marked variables.

    Consider now how can new %unmarked 
    variables be introduced in $\consis{\qelem_i}$. The only rule that locally introduces variables is $\mathbf{R}_{\Diamond}$, which applies to constraints of the form $\{x\col \standds C\}$. Notice that the normal form guarantees that any concept of the form $\standds C$ is the application of a modal operator to a basic concept $C\in\BCC$.
    There are at most $|\CC|$ different concepts of the form $\standds C$ and each can be applied at most once because the variable that triggers the rule does not play a role in its effect and no rule produces constraints of the form $x\col \standds C$ with $\standds C\notin \CC$. Therefore at most $|\CC|$ variables can be internally generated in $\consis{\qelem_i}$. Finally, the rules $\mathbf{R}_{r}$ and $\mathbf{R}_{r'}$ apply to named individuals and can introduce externally generated variables in $\consis{\qelem_i}$. Since there are at most $\size{\kb}$ elements for named individuals in $\mathbf{CG}$, each of which with $|\CC|$ internally generated variables, then $\size{\kb}^2$ variables can be externally introduced in $\consis{\qelem_i}$.

    Now, consider the elements that are generated via a global generating rule: Clearly, a new element $g$ produced by the $\mathbf{R}_{\exists}$ rule will have $\stvar{g}{*}=\stvar{\qelem_{\top}}{*}+1$ variables (notice that $\mathbf{R}_{r}$ and $\mathbf{R}_{r'}$ are never applicable to elements that are generated via a global generating rule).
    Since the variables from $\initialcs$ are copied to $g$ with their constraints, $g$ will still contain at most $|\CC|$ variables introduced by the $\mathbf{R}_{\Diamond}$ and an additional variable from the rule $\mathbf{R}_{\exists}$.

    Hence, we can conclude that every element $\qelem\in\mathbf{SC}$ has at most $2\size{\kb}^2$ variables. It should be clear that each variable can in turn be assigned to (a) each concept in $\CC$, (b) one individual in $\objC$, (c) each subformula in $\forC$ and (d) each standpoint in $\SC$, hence each variable has at most $\size{\kb}$ constraints. Consequently, there are at most $2\size{\kb}^3$ constraints in $\consis{\qelem}$.
\end{proof}

\begin{proof}[Proof of \Cref{theorem:termination}]\label{proof:termination}
    In view of Lemma \ref{lemma:num-elements-cs}, there are at most $3\size{\kb}^2$ elements in each completion graph constructed by the algorithm. As every global generating rule adds a new node, the number of applications of such rules ($\mathbf{R}_{\exists}$) is bounded by the same number.

    Now let us compute the number of applications of the rest of tableau rules. Since the rules $\mathbf{R}_{\preceq}$, $\mathbf{R}_{\sqcap}$, $\mathbf{R}_{\sqsubseteq}$, $\mathbf{R}_{\Box}$, $\mathbf{R}_{\Diamond}$, $\mathbf{R}_{g}$,
    $\mathbf{R}_{a}$, $\mathbf{R}_{r}$, $\mathbf{R}_{r'}$ and $\mathbf{R}_{\downarrow}$ produce one or more new constraints in an element, and from Lemma \ref{lemma:num-constraints-per-element} we know that there are at most $2\size{\kb}^3$ constraints in every element, then the number of applications of such rules per element is bounded by the same number.

    The only rule that does not produce new constraints is $\mathbf{R}_{\exists'}$. This rule can add, for each $\qelem$ with $(C,s,x)\in\elabel{\qelem}$, at most one quasi-role from every variable in every element. Recall that by the rules of the algorithm, no element is generated with more than one label. Since the bound on variables per object is $2\size{\kb}^2$ and the bound in the size of the domain is $3\size{\kb}^2$, then we have at most $6\size{\kb}^4$ rule applications.

    Finally, the number of applications of these rules during the execution of the algorithm is bounded by the bound on rule applications per element multiplied by the bound on elements, and together with the bound on $\mathbf{R}_{\exists}$ that gives us the total bound on tableau rule applications:
    \begin{linenomath*}
        $$ (6\size{\kb}^4)(3\size{\kb}^2) + (2\size{\kb}^3)(3\size{\kb}^2) + 3\size{\kb}^2 \leq (27\size{\kb}^6) $$
    \end{linenomath*}

\end{proof}

\subsection{Soundness and Completeness}\label{sec:app-soundness-completeness}

\begin{proof}[Proof of \Cref{theorem:soundness}]
    We will show that if there is a globally complete, coherent and clash-free completion graph $\mathbf{CG}$ for a $\SEL$ knowledge base $\kb$, then there is a quasi-model for $\kb$. If there is a quasi-model for $\kb$ it follows that $\kb$ is quasi-satisfiable, and by Theorem \ref{theorem:satisfiable-iff-quasisatisfiable}, if $\kb$ is quasi-satisfiable then it is satisfiable.

    Let $\mathbf{CG}=\tuple{\Delta,\consisf,\elabelf,\rolesf}$ be a globally complete, coherent and clash-free completion graph for $\kb$. Set $\mathcal{Q}=\tuple{\Delta,\consisf,\elabelf,\rolesf,\runsf}$, where $\runsf$ are all possible runs %and $\rolesf$ are all possible quasi-roles 
    on $\mathcal{Q}$. To show that $\mathcal{Q}$ is a quasi-model for $\kb$, we show that we can generate a run in $\mathcal{Q}$ with $r(\qelem)=v$ for each variable  $v$ in $\consisu{\qelem}$, with $\qelem\in\Delta$.
    \begin{description}
        \item[\ref{condition:run-standpoint}:] By \Cref{def:coherence} we have that if $r(\qelem)=v$, then for each $\qelem'\in\Delta$ there is some $v'$ such that $\stlabel{\qelem}{v}=\stlabel{\qelem'}{v'}$ such that we can set $r(\qelem')=v'$.
        \item [\ref{condition:run-role}:] Moreover, from the definition of a constraint graph we know that if $\tuple{\qelem', v', \qelem, v, R}\in\rolesf$ then $\stlabel{\qelem}{v}=\stlabel{\qelem'}{v'}$. Then, by the non-applicability of the $\mathbf{R}_{\downarrow}$ rule, we have that $(v' \col \exists R.C) \in\consisu{\qelem}$ if $(v\col C)\in\consisu{\qelem'}$. Thus, we can generate a run with $r(\qelem)=v$ and $r(\qelem')=v'$ also satisfying \ref{condition:run-standpoint}.
        \item [\ref{condition:run-existential}:] If $(v\col \exists R.C) \in\consisu{\qelem}$, then from the non-applicability of $\mathbf{R}_{\exists}$ there must be some $\qelem'\neq\qelem$ such that $(C,s,x)\in\elabel{\qelem'}$, $s=\stlabel{\qelem}{v}$ and $\tuple{\qelem, r(\qelem), \qelem', x, R}\in\rolesf$. It is clear that we can generate a run with $r(\qelem)=v$ and $r(\qelem')=v'$ also satisfying \ref{condition:run-standpoint} and \ref{condition:run-role}.
    \end{description}
    Hence we conclude that $\mathcal{Q}$ is a quasi-model for $\kb$.
\end{proof}

\begin{lemma}\label{lemma:same-axiom-per-standpoint}
    Let $\mathbf{CG}$ be a locally complete completion graph for $\kb$ produced by the algorithm, and let $\qelem, \qelem'$ be elements of $\mathbf{CG}$. For all variables $v$ in $\consis{\qelem}$ and $v'$ in $\consis{\qelem'}$ it is the case that if $\stlabel{{\qelem}}{v}=\stlabel{{\qelem'}}{v'}$ then $\{\phi \mid (v\col \phi)\in\consis{\qelem}\}=\{\phi\mid(v'\col \phi)\in\consis{\qelem'}\}$.
\end{lemma}

\begin{proof}

    We show that if $\stlabel{{\qelem}}{v}=\stlabel{{\qelem'}}{v'}$ and $(v\col \phi)\in\consis{\qelem}$ then $(v'\col \phi)\in\consis{\qelem'}$.

    \noindent If $(v\col \phi)\in\consis{\qelem}$ then clearly either (1) $\phi\in\kb$ or (2) $\phi\in\forC$.
    \begin{enumerate}
        \item If $(v\col \phi)\in\consis{\qelem}$ and $\phi\in\kb$. By the definition of a constraint system for $\kb$ we have $(v_*\col \phi)\in\consis{\qelem'}$, and since the normal form forces all axioms in $\kb$ to be of the form $\st\preceq\sp$ or $\standbs\psi$, we obtain $(v'\col \phi)\in\consis{\qelem'}$ from the non-applicability of $\mathbf{R}_{g}$.

        \item If $(v\col \phi)\in\consis{\qelem}$ and $\phi\in\forC$ but $\phi\notin\kb$
              \begin{enumerate}
                  \item It can only be that there is a formula $\standbs\phi\in\kb$
                  \item Notice that given (2) and (a), the constraint $(v\col \phi)\in\consis{\qelem}$ can only have been produced by a rule $\mathbf{R}_{\Box}$ or $\mathbf{R}_{\exists}$. We show that $\{(v\col \standbs\phi),(v\col \st)\}\subseteq\consis{\qelem}$:
                        \begin{description}
                            \item [Case 1:] $(v\col \phi)\in\consis{\qelem}$ was produced by $\mathbf{R}_{\Box}$. Then by the conditions of the rule $\{(v\col \standbs\phi),(v\col \st)\}\subseteq\consis{\qelem}$
                            \item [Case 2:] $(v\col \phi)\in\consis{\qelem}$ was produced by $\mathbf{R}_{\exists}$. Then $(v\col \phi)\in\consis{\qelem_{\top}}$. Then by \emph{Case 1} on $\qelem_{\top}$ we have $\{(v\col \standbs\phi),(v\col \st)\}\subseteq\consis{\qelem_{\top}}$ and by the same $\mathbf{R}_{\exists}$ rule also  $\{(v\col \standbs\phi),(v\col \st)\}\subseteq\consis{\qelem}$
                        \end{description}
                  \item By (b) and the non-applicability of the rule  $\mathbf{R}_{\Box}$ we have $(v'\col \phi)\in\consis{\qelem'}$ as desired.
              \end{enumerate}
    \end{enumerate}

\end{proof}

\begin{proof}[Proof of \Cref{theorem:completeness}]
    If $\kb$ is satisfiable then it is quasi-satisfiable (Theorem \ref{theorem:satisfiable-iff-quasisatisfiable}), and hence there is a quasi-model $\mathcal{Q}=\tuple{\Delta^q,\consisfq,\elabelf^q,\rolesf^q,\runsf^q}$ for $\kb$. We use $\mathcal{Q}$ as a guide and the tableau rules to construct a globally complete, coherent and clash-free completion tree $\mathbf{CG}=\tuple{\Delta,\consisf,\elabelf,\rolesf}$ for $\kb$. For the sake of better readability, let us  refer to the elements of $\Delta$ with $\qelemg, \qelemg', \dots$ and to the elements of $\Delta^q$ with $\qelem, \qelem', \dots$.

    % Say that a completion graph $\mathbf{CG}$ for $\kb$ is $\mathcal{Q}$-compatible if the following holds:
    % \begin{itemize}[label={-}]
    %     \item There is a relation $\mu \subseteq \Delta\times\Delta^q$ such that, for all $\qelemg\in\Delta$ and $\qelem\in\Delta^{q}$, $(\qelemg,\qelem)\in\crel$ if:
    %     \begin{itemize}[leftmargin=0.8cm, label={-}]
    %         \item if $(x\col a)\in\consis{\qelemg}$ then $(v\col a)\in\consisq{\qelem}$ and
    %         \item $\elabel{\qelemg}\subseteq\elabelq{\qelem}$.
    %     \end{itemize}
    %     \item For each $\qelemg\in\Delta$ there is at least one pair $(\qelemg,\qelem)\in\crel$.
    %     %\item We use $\mu$ from the set of elements in $\Delta$ to $\Delta^q$
    %     \item For each pair $(\qelemg,\qelem)$ in $\crel$, there is a (total) surjective function $\cfuncf{\qelemg,\qelem}$ from the set of variables in $\consisq{\qelem}$ to the set of variables in $\consis{\qelemg}$ such that for $\cfunc{\qelemg,\qelem}{v}=x$ 
    %     \begin{itemize}[leftmargin=0.8cm, label={-}]
    %       %  \item $\stlabel{\qelemg}{x}\subseteq\stlabel{\qelem}{v}$ and
    %         \item  if $(x\col \st)\in\consis{\qelemg}$ then $(v\col \st)\in\consisq{\qelem}$ and
    %         \item  if $(x\col \Phi)\in\consis{\qelemg}$ then $(v\col \Phi)\in\consisq{\qelem}$.
    %     \end{itemize}
    %     \item If $\tuple{\qelemg, x, \qelemg', x', R}\in\rolesf$, then there are some $(\qelemg,\qelem), (\qelemg',\qelem')\in\crel$ with $\cfunc{\qelemg,\qelem}{y}=x$ and $\cfunc{\qelemg',\qelem'}{y'}=x'$ and $\tuple{\qelem, y, \qelem', y', R}\in\rolesf^q$ 
    % \end{itemize}

    \begin{claim}
        The completion graph $\mathbf{CG}_{I}\!=\!\tuple{\Delta,\consisf,\elabelf,\rolesf}$ for $\kb$ s.t.
        \begin{itemize}
            \item $\Delta=\{\qelemg_{\top}\}\cup\{\qelemg_{a}\mid a\in\objC\}$,
            \item $\consis{\qelemg_{\top}}=\initialcs$,
            \item $\consis{\qelemg_{a}}=\initialcs \cup \{(x_{\st}\col a)\mid x_{\st}\!\in\!\stvar{\initialcs}{*} \}$ for each $a\in\objC$,
            \item $\elabel{\qelemg}=\emptyset$ for each $\qelemg\in\Delta$, and
            \item $\rolesf=\emptyset$
        \end{itemize}
        is $\mathcal{Q}$-compatible.
    \end{claim}

    Recall that $\initialcs= \{(x_{\st}\col *), (x_{\st}\col \top), (x_{\st}\col \phi),  (x_{\st}\col \st) \mid \phi\in\kb, \st\in\SC \}$. By the definition of a completion graph, $\Delta^q$ is non-empty. It is clear that for all elements $\qelem\in\Delta^q$ we have $(\qelemg_{\top},\qelem)\in\crel$. Moreover, by the definition of a quasi-model, for each $a\in\objC$ there is a unique quasi-element $\qelem_a\in\Delta^q$ such that $(v\col a)\in\consisq{\qelem_a}$ for all variables $v$ in $\consisq{\qelem_a}$. Set $(\qelemg_a,\qelem_a)\in\crel$. From the former and the fact that for all $\qelemg\in\Delta$ we have $\elabel{\qelemg}=\emptyset$, it is clear that $\crel$ is as required. Notice that by definition $\initialcs\subseteq\elabelq{\qelem}$ for all $\qelem\in\Delta^q$ and if $(x\col a)\in\consis{\qelemg_a}$ then also $(v\col a)\in\consisq{\qelem_a}$. Then we can set $\cfunc{\qelemg,\qelem}{v_{\st}}=x_{\st}$ for each $(\qelemg,\qelem)\in\crel$, $x_{\st}$ in $\consis{\qelemg}$ and $v_{\st}$ in $\qelem$. Moreover, for $v$ in $\qelem$ there is some $v_{\st}$ such that $\stlabel{\qelem}{v}=\stlabel{\qelem}{v_{\st}}$, thus we can set $\cfunc{\qelemg,\qelem}{v}=\cfunc{\qelemg,\qelem}{v_{\st}}$. It should be clear that $\cfuncf{\qelemg,\qelem}$ is as required.

    \begin{claim}
        If a completion graph $\mathbf{CG}$ for $\kb$ is $\mathcal{Q}$-compatible and $\mathbf{CG}'$ is the result of an application of a rule $\mathbf{R}$ to $\mathbf{CG}$, then $\mathbf{CG}'$ is $\mathcal{Q}$-compatible as well.
    \end{claim}

    Let $\mathbf{CG}$ be an $\mathcal{Q}$-compatible completion graph, $\qelemg$ an element in $\mathbf{CG}$ and let $\crel$ and for all $(g,\qelem)\in\crel$ let $\cfuncf{\qelemg,\qelem}$ be the functions supplied by the definition of $\mathcal{Q}$-compatibility. Let us consider all the cases for $\mathbf{R}$.

    \begin{description}[itemsep=0.2cm]
        \item[$\mathbf{R}_{\preceq}\ $] Suppose that the rule $\mathbf{R}_{\preceq}$ is applicable to the constraints $\{(x\col \st\preceq \sp), (x'\col \st)\}\subseteq\consis{\qelemg}$ with $(x'\col \sp)\notin\consis{\qelemg}$. Let $(\qelemg,\qelem)\in\crel$ and $y$ and $y'$ be variables in $\consisq{\qelem}$ such that $\cfunc{\qelemg,\qelem}{y} = x$ and $\cfunc{\qelemg,\qelem}{y'} = x'$. Then we have $\{(y\col \st\preceq \sp),(y'\col \st)\}\subseteq\consisq{\qelem}$. The non-applicability of $\mathbf{R}_{\preceq}$ to $\consisq{\qelem}$ means that $(y' \col \sp) \in \consisq{\qelem}$. The application of the $\mathbf{R}_{\preceq}$ rule adds $(x' \col \sp) \in \consis{\qelemg}$. Hence, the relation $\crel$ and the function $\cfuncf{\qelemg,\qelem}$ are as required for the resulting completion graph $\mathbf{CG}'$.

        \item[$\mathbf{R}_{\sqcap}\ $] Suppose that the rule $\mathbf{R}_{\sqcap}$ is applicable to the constraints $\{x \col C, x\col D\} \subseteq\consis{\qelemg}$. Let $(\qelemg,\qelem)\in\crel$ and $y$ be a variable in $\consisq{\qelem}$ such that  $\cfunc{\qelemg,\qelem}{y} = x$. Then we have $\{y \col C, y\col D\} \subseteq \consisq{\qelem}$. The non-applicability of $\mathbf{R}_{\sqcap}$ to $\consisq{\qelem}$ means that $(y \col C \sqcap D) \in \consisq{\qelem}$. The application of the $\mathbf{R}_{\sqcap}$ rule adds $(x \col C \sqcap D) $ to $\consis{\qelemg}$. Hence, the relation $\crel$ and the function $\cfuncf{\qelemg,\qelem}$ are as required for the resulting completion graph $\mathbf{CG}'$.

        \item[$\mathbf{R}_{\sqsubseteq}\ $] Suppose that the rule $\mathbf{R}_{\sqsubseteq}$ is applicable to the constraints $\{x\col C, x\col C\sqsubseteq D\} \subseteq\consis{\qelemg}$. Let $(\qelemg,\qelem)\in\crel$ and $y$ be a variable in $\consisq{\qelem}$ such that $\cfunc{\qelemg,\qelem}{y} = x$. Then we have $\{y \col C, y\col C\sqsubseteq D\} \subseteq \consisq{\qelem}$. The non-applicability of $\mathbf{R}_{\sqsubseteq}$ to $\consisq{\qelem}$ means that $(y \col D) \in \consisq{\qelem}$. The application of the $\mathbf{R}_{\sqsubseteq}$ rule adds $(x \col D) $ to $\consis{\qelemg}$. Hence, the relation $\crel$ and the function $\cfuncf{\qelemg,\qelem}$ are as required for the resulting completion graph $\mathbf{CG}'$.

        \item[$\mathbf{R}_{\Box}\ $] Suppose that the rule $\mathbf{R}_{\Box}$ is applicable to the constraints $\{x\col \standbs \Phi, x'\col \st\}\subseteq\consis{\qelemg}$ with $(x \col \Phi)\notin\consis{\qelemg}$. Let $(\qelemg,\qelem)\in\crel$ and $y$ and $y'$ be variables in $\consisq{\qelem}$ such that $\cfunc{\qelemg,\qelem}{y} = x$ and $\cfunc{\qelemg,\qelem}{y'} = x'$. Then we have $\{y\col \standbs \Phi,\ y'\col \st\}\subseteq\consisq{\qelem}$. The non-applicability of $\mathbf{R}_{\Box}$ to $\consisq{\qelem}$ means that $(y' \col \Phi) \in \consisq{\qelem}$. The application of the $\mathbf{R}_{\Box}$ rule adds $(x' \col \Phi) $ to $\consis{\qelemg}$. Hence, the relation $\crel$ and the function $\cfuncf{\qelemg,\qelem}$ are as required for the resulting completion graph $\mathbf{CG}'$.

        \item[$\mathbf{R}_{g}\ $] Suppose that the rule $\mathbf{R}_{g}$ is applicable to the constraint $\{x \col \mathbf{G}\}\subseteq\consis{\qelemg}$ with $(x' \col \mathbf{G})\notin\consis{\qelemg}$ for some $x'$ in $\consis{\qelemg}$. Let $(\qelemg,\qelem)\in\crel$ and $y$ and $y'$ be variables in $\consisq{\qelem}$ such that $\cfunc{\qelemg,\qelem}{y} = x$ and $\cfunc{\qelemg,\qelem}{y'} = x'$. Then we have $\{y\col \mathbf{G}\} \subseteq \consisq{\qelem}$. The non-applicability of $\mathbf{R}_{g}$ to $\consisq{\qelem}$ means that $(y' \col \mathbf{G}) \in \consisq{\qelem}$. The application of the $\mathbf{R}_{g}$ rule adds $(x' \col \mathbf{G}) $ to $\consis{\qelemg}$. Hence, the relation $\crel$ and the function $\cfuncf{\qelemg,\qelem}$ are as required for the resulting completion graph $\mathbf{CG}'$.

        \item[$\mathbf{R}_{a}\ $] Suppose that the rule $\mathbf{R}_{a}$ is applicable to the constraints $\{x\col a, x\col C(a)\} \subseteq\consis{\qelemg}$. Let $(\qelemg,\qelem)\in\crel$ and $y$ be a variable in $\consisq{\qelem}$ such that $\cfunc{\qelemg,\qelem}{y} = x$. Then we have $\{y \col a, y\col C(a)\} \subseteq \consisq{\qelem}$. The non-applicability of $\mathbf{R}_{a}$ to $\consisq{\qelem}$ means that $(y \col C) \in \consisq{\qelem}$. The application of the $\mathbf{R}_{a}$ rule adds $(x \col C) $ to $\consis{\qelemg}$. Hence, the relation $\crel$ and the function $\cfuncf{\qelemg,\qelem}$ are as required for the resulting completion graph $\mathbf{CG}'$.

        \item[$\mathbf{R}_{\Diamond}\ $] Suppose that the rule $\mathbf{R}_{\Diamond}$ is applicable to the constraint $(x\col \standds C)\in\consis{\qelemg}$ with no $x'$ in $\consis{\qelemg}$ such that $\{x' \col \st,\ x' \col C\}\subseteq \consis{\qelemg}$. Let $(\qelemg,\qelem)\in\crel$ and $y$ be a variable in $\consisq{\qelem}$ such that $\cfunc{\qelemg,\qelem}{y} = x$. Then we have $(y\col \standds C)\in\consisq{\qelem}$. The non-applicability of $\mathbf{R}_{\Diamond}$ to $\consisq{\qelem}$ means that there exists $y'$ in $\consisq{\qelem}$ such that $\{y' \col \st,\ y' \col C\}\subseteq\consisq{\qelem}$. The application of the $\mathbf{R}_{\Diamond}$ rule to $\consis{\qelemg}$ creates a fresh variable $x'$  and sets $\{x' \col \st,\ x' \col C\}\subseteq \consis{\qelemg}$. Then we define $\cfuncfp{\qelemg,\qelem}$ as the update of $\cfuncf{\qelemg,\qelem}$ with $\cfuncp{\qelemg,\qelem}{y'} = x'$ (notice that  if $(x'\col \st)\in\consis{\qelemg}$ then $(y'\col \st)\in\consisq{\qelem}$). Hence, the relation $\crel$ and the function $\cfuncfp{\qelemg,\qelem}$ are as required for the resulting completion graph $\mathbf{CG}'$.

        \item[$\mathbf{R}_{\exists}\ $] Suppose that the rule $\mathbf{R}_{\exists}$ is applicable to the constraint $(x\col \exists R.C) \in\consis{\qelemg}$ since there is no $\qelemg'\in\Delta$ such that $(C,\stlabel{\qelemg}{x},x')\in\elabel{\qelemg'}$, $\langle \qelemg, x, \qelemg', x', R\rangle\in\rolesf$ and $\qelemg'\neq \qelemg$. Let $(\qelemg,\qelem)\in\crel$ and $y$ be a variable in $\consisq{\qelem}$ such that $\cfunc{\qelemg,\qelem}{y} = x$. Then we have $(y\col \exists R.C) \in\consisq{\qelem}$. The non-applicability of $\mathbf{R}_{\exists}$ to $\consisq{\qelem}$ means that there exists $\qelem^q$ in $\Delta^q$ such that $(C,s,y')\in\elabelq{\qelem^q}$ with $s=\stlabel{\qelem}{y}$ and $\langle \qelem, y, \qelem', y', R\rangle\in\rolesf$. This implies that $\{y'\col C,\ y'\col \top\}\cup\{y'\col \st \mid (y\col \st)\in\consisq{\qelem}, \st\in\SC \}\subseteq\consisq{\qelem^q}$. The rule application of $\mathbf{R}_{\exists}$ to $\consis{\qelemg}$ generates an element $\qelemg'$ with $\elabel{\qelemg'}=(C,\stlabel{\qelemg}{x},x')$, $\rolesf\eqdef \rolesf\cup \{\langle \qelemg, x, \qelemg', x', R\rangle\}$ and $\consis{\qelemg'}=\consis{\qelemg_{\top}}\cup\{x'\col C,\ x'\col \top\}\cup\{x'\col \st \mid (x\col \st)\in\consis{\qelemg}, \st\in\SC \}$. We define $\crel'$ as the extension of $\crel$ such that $(\qelemg',\qelem')\in\crel'$ for all $\qelem'\in\Delta^q$ with $(C,s,y')\in\elabelq{\qelem'}$. Note that there is at least one element, $\qelem^q$, such that $(\qelemg',\qelem^q)\in\crel'$.

            Now, we must define $\cfuncf{\qelemg',\qelem'}$ for each $(\qelemg',\qelem')\in\crel'$. It is clear that we can set $\cfunc{\qelemg',\qelem'}{y'}=x'$. For the rest of variables $x_{\st}\in\stvar{\qelemg'}{*}$ such that $x_{\st}\neq x'$, we recall that $\initialcs= \{(x_{\st}\col *), (x_{\st}\col \top), (x_{\st}\col \phi),  (x_{\st}\col \st) \mid \phi\in\kb, \st\in\SC \}$ and that by the definition of a constraint system $\initialcs\subseteq\consisq{\qelem'}$. Then, we can set $\cfunc{\qelemg',\qelem'}{y_{\st}}=x_{\st}$ for each $x_{\st}\in\stvar{\qelemg'}{*}$ with $y_{\st}$ in $\consisq{\qelem^q}$ and for every unassigned $y''$ in $\consisq{\qelem^q}$ there is some $y_{\st}$ such that $\stlabel{\qelem^q}{y''}=\stlabel{\qelem^q}{y_{\st}}$ (by \Cref{def:coherence}) and thus we set $\cfunc{\qelemg',\qelem'}{y''}=x_{\st}$.

            Again, $\crel'$ and each $\cfuncf{\qelemg',\qelem'}$ is as required for the resulting completion graph $\mathbf{CG}'$:
            \begin{itemize}[label={-}]
                \item $\elabel{\qelemg'}\subseteq\elabelq{\qelem'}$,
                \item  for $x\in\stvar{\qelemg'}{*}$ and $\cfunc{\qelemg',\qelem'}{y}=x$, if $(x\col \st)\in\consis{\qelemg'}$ then $(y\col \st)\in\consisq{\qelem'}$,
                \item  for $x\in\stvar{\qelemg'}{*}$ and $\cfunc{\qelemg',\qelem'}{y}=x$, if $(x\col \Phi)\in\consis{\qelemg'}$ then $(y\col \Phi)\in\consisq{\qelem'}$,
                \item  for $\langle \qelemg, x, \qelemg', x', R\rangle\in\rolesf$ we have $\langle \qelem, y, \qelem^q, y', R\rangle\in\rolesf^q$ with $\cfunc{\qelemg',\qelem^q}{y'}=x'$
            \end{itemize}

        \item[$\mathbf{R}_{\downarrow}\ $]
            Suppose that the rule $\mathbf{R}_{\downarrow}$ is applicable since $(x\col C)\in \consis{\qelemg}$ and $\langle \qelemg', x', \qelemg, x, R\rangle\in\rolesf$, but $(x' \col \exists R.C)\notin \consis{\qelemg'}$.

            %    First, notice that, since $\mathbf{CG}$ is produced by the tableau algorithm, there is at most one element $\qelemg'\in\Delta$ with $\elabel{\qelemg'}=\{(C,\stlabel{\qelemg}{x},x')\}$ (see the tableau rules \Cref{fig:rules}). Moreover, by the construction of $\crel$ (notably by the rule $\mathbf{R}_{\exists}$) for all $\qelem'\in\Delta^q$ such that $(C,s,y')\in\elabelq{\qelem'}$ we have $(\qelemg',\qelem')\in\crel'$. Let $\upepsilon_{\qelemg'}=\{\qelem'\mid(\qelemg',\qelem')\in\crel'\}$.

            Let $(\qelemg,\qelem),(\qelemg',\qelem')\in\crel$, $y$ be a variable in $\consisq{\qelem}$ such that $\cfunc{\qelemg,\qelem}{y} = x$ and $y'$ a variable in $\consisq{\qelem'}$ such that $\cfunc{\qelemg',\qelem'}{y'} = x'$. Then we have $(y\col C) \in\consisq{\qelem}$ and $\langle \qelem', y', \qelem, y, R\rangle\in\rolesf^q$. By the non-applicability of the $\mathbf{R}_{\downarrow}$ rule on $\mathcal{Q}$ we have that $(y'\col \exists R.C)\in\consisq{\qelem'}$

            On the other hand, the application of the rule $\mathbf{R}_{\downarrow}$ adds $(x \col \exists R.D)$ to $\consis{\qelemg}$. Consequently, the relation $\crel$ and the functions $\cfuncf{\qelemg,\qelem}$ and $\cfuncf{\qelemg',\qelem'}$ are as required for the resulting completion graph $\mathbf{CG}'$.

        \item[$\mathbf{R}_{r}\ $]
            Suppose that the rule $\mathbf{R}_{r}$ is applicable to the constraints $\{x \col a,\ x \col R(a,b)\}\subseteq \consis{\qelemg}$ since $\langle \qelemg, x, \qelemg', x, R\rangle\notin\rolesf$ for some $\qelemg'\in\Delta$ with $(x'\col b)\in\consis{\qelemg'}$.

            First, notice that, since $\mathbf{CG}$ is produced by the tableau algorithm, there is exactly one element $\qelemg\in\Delta$ with $(x\col a)\in\consis{\qelemg}$ and one element $\qelemg'\in\Delta$ with $(x'\col b)\in\consis{\qelemg'}$ (see the initialisation of the tableau and its rules \Cref{fig:rules}). Moreover, by the definition of a quasi-model, there is also exactly one element $\qelem\in\Delta^q$ with $(x\col a)\in\consisq{\qelem}$ and one element $\qelem'\in\Delta^q$ with $(x'\col b)\in\consisq{\qelem'}$. From this and the construction of $\crel$, we have only two pairs $(\qelemg,\qelem),(\qelemg',\qelem')\in\crel$ related to this rule.

            Let $y$ be a variable in $\consisq{\qelem}$ such that $\cfunc{\qelemg,\qelem}{y} = x$. Then we have $\{y\col a,\ y\col R(a,b)\}\subseteq\consisq{\qelem}$. By the non-applicability of the  $\mathbf{R}_{r}$ rule, we also have $\langle \qelem, y, \qelem', y, R\rangle\in\rolesf^q$. And, by the definition of a completion graph $\stlabel{\qelem}{y}=\stlabel{\qelem'}{y}$.
            Thus we have $\{y \col \top\}\ \cup\ \{y\col \st \mid \st\in\stlabel{\qelem}{y} \}\subseteq\consis{\qelem'}$ and $\rolesf\eqdef \rolesf\cup \{\langle \qelem, y, \qelem', y, R\rangle\}$.

            By the application of $\mathbf{R}_{r}$ on $\mathbf{CG}$, we obtain $\langle \qelemg, x, \qelemg', x, R\rangle\in\rolesf$ and $\{x \col \top\}\ \cup\ \{x\col \st \mid \st\in\stlabel{\qelemg}{x} \}\subseteq\consis{\qelemg'}$ and $\rolesf\eqdef \rolesf\cup \{\langle \qelemg, x, \qelemg', x, R\rangle\}$.
            Then we define $\cfuncfp{\qelemg',\qelem'}$ as the update of $\cfuncf{\qelemg',\qelem'}$ with $\cfuncp{\qelemg',\qelem'}{y} = x$. Hence, the relation $\crel$ and the functions $\cfuncfp{\qelemg',\qelem'}$ and $\cfuncf{\qelemg,\qelem}$ are as required for the resulting completion graph $\mathbf{CG}'$.

        \item[$\mathbf{R}_{r'}\ $]
            Suppose that the rule $\mathbf{R}_{r'}$ is applicable to the constraints $\{x \col b,\ x \col R(a,b)\}\subseteq \consis{\qelemg}$ since $\langle \qelemg', x, \qelemg, x, R\rangle\notin\rolesf$ for some $\qelemg'\in\Delta$ with $(x'\col a)\in\consis{\qelemg'}$.

            First, notice that, since $\mathbf{CG}$ is produced by the tableau algorithm, there is exactly one element $\qelemg\in\Delta$ with $(x\col b)\in\consis{\qelemg}$ and one element $\qelemg'\in\Delta$ with $(x'\col a)\in\consis{\qelemg'}$ (see the initialisation of the tableau and its rules \Cref{fig:rules}). Moreover, by the definition of a quasi-model, there is also exactly one element $\qelem\in\Delta^q$ with $(x\col b)\in\consisq{\qelem}$ and one element $\qelem'\in\Delta^q$ with $(x'\col a)\in\consisq{\qelem'}$. From this and the construction of $\crel$, we have only two pairs $(\qelemg,\qelem),(\qelemg',\qelem')\in\crel$ related to this rule.

            Let $y$ be a variable in $\consisq{\qelem}$ such that $\cfunc{\qelemg,\qelem}{y} = x$. Then we have $\{y\col b,\ y\col R(a,b)\}\subseteq\consisq{\qelem}$. By the non-applicability of the  $\mathbf{R}_{r'}$ rule, we also have $\langle \qelem', y, \qelem, y, R\rangle\in\rolesf^q$. And, by the definition of a completion graph $\stlabel{\qelem}{y}=\stlabel{\qelem'}{y}$.
            Thus we have $\{y \col \top\}\ \cup\ \{y\col \st \mid \st\in\stlabel{\qelem}{y} \}\subseteq\consis{\qelem'}$ and $\rolesf\eqdef \rolesf\cup \{\langle \qelem', y, \qelem, y, R\rangle\}$.

            By the application of $\mathbf{R}_{r'}$ on $\mathbf{CG}$, we obtain $\langle \qelemg', x, \qelemg, x, R\rangle\in\rolesf$ and $\{x \col \top\}\ \cup\ \{x\col \st \mid \st\in\stlabel{\qelemg}{x} \}\subseteq\consis{\qelemg'}$ and $\rolesf\eqdef \rolesf\cup \{\langle \qelemg', x, \qelemg, x, R\rangle\}$.
            Then we define $\cfuncfp{\qelemg',\qelem'}$ as the update of $\cfuncf{\qelemg',\qelem'}$ with $\cfuncp{\qelemg',\qelem'}{y} = x$. Hence, the relation $\crel$ and the functions $\cfuncfp{\qelemg',\qelem'}$ and $\cfuncf{\qelemg,\qelem}$ are as required for the resulting completion graph $\mathbf{CG}'$.

        \item[$\mathbf{R}_{\exists'}\ $] Suppose that the rule $\mathbf{R}_{\exists'}$ is applicable to a constraint $(x \col \exists R.C)\in \consis{\qelemg}$ for which there is a $\qelemg'$ with $(C,\stlabel{\qelemg}{x},x')\in\elabel{\qelemg'}$ and $\qelemg\neq\qelemg'$, since $\langle \qelemg, x, \qelemg'', x'', R\rangle\notin\rolesf$ for some $\qelemg'', x''$ with $(x'' \col C)\in \consis{\qelem''}$.%, then set $\rolesf\eqdef \rolesf\cup \{\langle \qelem, x, \qelem', x', R\rangle\}$.

            Let $(\qelemg,\qelem)\in\crel$, let $y$ be a variable in $\consisq{\qelem}$ such that $\cfunc{\qelemg,\qelem}{y} = x$. Then we have $(y \col \exists R.C)\in \consis{\qelem}$, and by the non-applicability of the $\mathbf{R}_{\exists'}$ rule to $\mathcal{Q}$, there must be some $\langle \qelem, y, \qelem', y', R\rangle\in\rolesf^q$ for some $\qelem', y'$ with $(C,\stlabel{\qelem}{y},y')\in\elabel{\qelem'}$.
            By the application of the $\mathbf{R}_{\exists'}$ rule on $\mathbf{CG}$, we obtain $\rolesf\eqdef \rolesf\cup \{\langle \qelemg, x, \qelemg', x', R\rangle\}$. Then the relation $\crel$ and the functions $\cfuncfp{\qelemg',\qelem'}$ and $\cfuncf{\qelemg,\qelem}$ are as required for the resulting completion graph $\mathbf{CG}'$.

            Specifically notice that since $\langle \qelemg, x, \qelemg', x', R\rangle\in\rolesf$ there must be some $(\qelemg,\qelem), (\qelemg',\qelem')\in\crel$ with $\cfunc{\qelemg,\qelem}{y}=x$ and $\cfunc{\qelemg',\qelem'}{y'}=x'$ and $\tuple{\qelem, y, \qelem', y', R}\in\rolesf^q$. We already have that $(\qelemg,\qelem)\in\crel$ and $\cfunc{\qelemg,\qelem}{y} = x$. Moreover, by the $\mathbf{R}_{\exists}$ rule we have that for all $\qelemg''$ with $(C,\stlabel{\qelemg}{x},x')\in\elabel{\qelemg''}$ and all $\qelem''$ with $(C,\stlabel{\qelem}{y},y')\in\elabel{\qelem''}$, $(\qelemg'',\qelem'')\in\crel$. Thus we have $(\qelemg',\qelem')\in\crel$. Moreover, we also know from the application of the $\mathbf{R}_{\exists}$ rule that $\cfunc{\qelemg',\qelem'}{y'} = x'$. Hence there are some $(\qelemg,\qelem), (\qelemg',\qelem')\in\crel$ with $\cfunc{\qelemg,\qelem}{y}=x$ and $\cfunc{\qelemg',\qelem'}{y'}=x'$ such that $\langle \qelem, y, \qelem', y', R\rangle\in\rolesf^q$ as required. With this, the claim is proved.

    \end{description}

    Now, returning to the proof of the completeness theorem, we show that it
    follows from the claims above. Notice that $\mathbf{CG}_{I}$ is the initial completion graph produced by the algorithm for $\kb$ and that we have shown that it is $\mathcal{Q}$-compatible.
    By the second claim, the completion rules can be applied in such a way that
    the resulting completion graphs are $\mathcal{Q}$-compatible. According to Theorem \ref{theorem:termination} (Termination), we then eventually construct a globally complete $\mathcal{Q}$-compatible completion graph $\mathbf{CG}$.

    Let us now show that $\mathbf{CG}$ is clash-free. Suppose otherwise. Then there is an element $\qelemg$ in $\mathbf{CG}$ and a variable $x$ such that $(x\col\bot)\in\consis{\qelemg}$. Let $\crel$ be the relation supplied by the definition of $\mathcal{Q}$-compatibility. Then we must have some $\qelem\in\Delta^q$ with $(\qelemg,\qelem)\in\crel$ and some function $\cfuncf{\qelemg,\qelem}$ such that $(\cfunc{\qelemg,\qelem}{x}\col\bot)\in\consisq{\qelem}$, which is a contradiction because $\mathcal{Q}$ is a quasi-model.

    It remains to show that $\mathbf{CG}$ is coherent. For the first point, we may just observe that we initialise the algorithm with a unique element $\qelem_a\in\Delta$ for each $a\in\objC$ such that $(v_{*}\col a)\in\consisu{\qelem_a}$. Moreover, by the non-applicability of the $\mathbf{R}_{\downarrow}$ rule, we have that $(v\col a)\in\consisu{\qelem_a}$ for all variables $v$ in $\consisu{\qelem_a}$. Since no rule in \Cref{fig:rules} can propagate constraints of the form $(v\col a)$ to other elements, the first condition is satisfied. For the second condition, from \Cref{lemma:same-standpoints} it follows that for each $v$ in $\consis{\qelem}$, every $\consis{\qelem'}$ contains some $v'$ such that $\stlabel{\qelem}{v}=\stlabel{\qelem'}{v'}$ as desired. Finally, from \Cref{lemma:same-axiom-per-standpoint} it follows that for each $\consis{\qelem}$ and $\consis{\qelem'}$, if $(v\col\phi)\in\consis{\qelem}$ then $(v'\col\phi)\in\consis{\qelem'}$ for all $v'$ with $\stlabel{\qelem}{v}=\stlabel{\qelem'}{v'}$ as desired and we can thus conclude that $\mathbf{CG}$ is coherent.

\end{proof}

\section{Proofs for \Cref{sec:intractable-extensions}}

\newcommand{\SELO}{\SEL ?}
\begin{theorem}
    Satisfiability of $\SEL$ TBoxes with $*$ as the only occurring standpoint name and one distinguished rigid role $\dot{R}$ is \coNP-hard.
    \begin{proof}
        We reduce the \NP-hard problem SAT to TBox unsatisfiability.
        Assume an instance $\phi=\clause_1 \land \ldots \land \clause_n$ of SAT containing $n$ clauses $\clause_j$ (disjunctions of literals) over the propositional variables \mbox{$P = \set{ p_1,\ldots, p_k }$}.

        We construct the following $\SELO$ TBox $\T_\phi$ (of polynomial size):
        \begin{align}
            \top                                                  & \sqsubseteq \exists U. L_0                                                                                                                    \label{lstart}                                                                                    \\
            L_{i-1}                                               & \sqsubseteq \exists \dot{R}.(T_{p_i} \sqcap L_{i} ) \sqcap \exists \dot{R}. (T_{\neg p_i} \sqcap L_{i})                                                      & \text{ for all } 1\leq i\leq k      \label{lnext}                                \\
            L_{i} \sqcap T_{p_i}                                  & \sqsubseteq \standball ( L_{i} \sqcap T_{p_i} )                                                                                                              & \text{ for all } 1\leq i\leq k                                     \label{ltrue} \\
            L_{i} \sqcap T_{\neg p_i}                             & \sqsubseteq \standball ( L_{i} \sqcap T_{\neg p_i} )                                                                                                         & \text{ for all } 1\leq i\leq k      \label{lfalse}                               \\
            L_k                                                   & \sqsubseteq \standdall\!\mathit{Select}                                                                        \label{sstart}                                                                                                                   \\
            \exists \dot{R}.(T_{p_i} \sqcap \mathit{Select})      & \sqsubseteq (T_{p_i} \sqcap \mathit{Select})                                                                                                                 & \text{ for all } 1\leq i\leq k                       \label{strue}               \\
            \exists \dot{R}.(T_{\neg p_i} \sqcap \mathit{Select}) & \sqsubseteq (T_{\neg p_i} \sqcap \mathit{Select})                                                                                                            & \text{ for all } 1\leq i\leq k  \label{sfalse}                                   \\
            T_\ell                                                & \sqsubseteq T_{\clause_j}                                                                                                                                    & \text{ for all } \ell \in \clause_j \label{clause}                               \\
            T_{\clause_1} \sqcap \ldots \sqcap T_{\clause_n}      & \sqsubseteq \bot  \label{disjoint}
        \end{align}
        We conclude the proof by showing that $\phi$ is satisfiable iff $\T_\phi$ is unsatisfiable.
        \begin{description}
            \item[\normalfont``if'':]
                We show the contrapositive.
                Let $\phi$ be unsatisfiable.
                We construct a model \mbox{$\dlstruct= \tuple{\Dom, \Precs, \sigma, \gamma}$} for $\T_\phi$ as follows.
                \begin{align*}
                    \Dom   & = \set{ w\in\set{0,1}^* \guard \abs{w}\leq k } \\
                    \Precs & = 2^P
                \end{align*}
                That is, the interpretation domain contains all words $w$ over $\set{0,1}$ of length at most $k$ (including the empty word $\nil$).
                Roughly, each $w$ encodes a partial interpretation of $P$ where $w_i$, the $i$-th symbol in $w$, encodes whether $p_i$ is true ($w_i=1$) or false ($w_i=0$) or undefined ($\abs{w}<i$).

                Finally, for each $Q\subseteq P$, the DL interpretation $\gamma(Q)=\tuple{\Dom,\intf}$ is given by
                \begin{align*}
                    \interprets{U}               & = \Dom\times\set{ \nil }                                                                           \\
                    \interprets{\dot{R}}         & = \set{ \tuple{w,w0}, \tuple{w,w1} \guard w,w0,w1\in\Dom }                                         \\
                    \interprets{L_i}             & = \set{ w\in\Dom \guard \abs{w}=i }                                                                \\
                    \interprets{T_{p_i}}         & = \set{ w\in\Dom \guard w_i=1 } \cup \set{ w\in\Dom \guard w\in\prefixes(w^Q), \abs{w}<i, w^Q_i=1} \\
                    \interprets{T_{\neg p_i}}    & = \set{ w\in\Dom \guard w_i=0 } \cup \set{ w\in\Dom \guard w\in\prefixes(w^Q), \abs{w}<i, w^Q_i=0} \\
                    \interprets{\mathit{Select}} & = \prefixes(w^Q)                                                                                   \\
                    \interprets{T_{\clause_j}}   & = \bigcup_{\ell\in\clause_j}\interprets{T_{\ell}}
                \end{align*}
                Where the word $w^Q$ of length $k$ encodes the valuation $Q$ via
                \[
                    w^Q_i               = \begin{cases}
                        0 & \text{ if } p_i\notin Q \\
                        1 & \text{ otherwise}
                    \end{cases}
                \]
                and $\prefixes(w)=\set{v\in\set{0,1}^* \guard \exists u\in\set{0,1}^*: w=vu}$ denotes the set of all prefixes of $w\in\set{0,1}^*$.
                %Observe that $Q\models p_i$ iff $w^Q\in T_{p_i}$, and $Q\not\models p_i$ iff $w^Q\in T_{\neg p_i}$.

                We now show that $\dlstruct\models\T_\phi$.
                Unless declared otherwise, assume that $\struct=\gamma(Q)$ is for an arbitrary $Q\subseteq P$.

                We note that the interpretations of the $L_i$ ($0\leq i\leq k$) and $T_{\clause_j}$ ($1\leq j\leq n$) is the same across precisifications, and for $T_{p_i}$ and $T_{\neg p_i}$ their extensions agree on all words of length at least $i$.
                \begin{itemize}
                    \item (\ref{lstart}): By definition.
                    \item (\ref{lnext}): Let $w\in\interprets{L_{i-1}}$.
                          Then $\abs{w}=i-1$.
                          In particular, since $i-1<k$, we have $w0,w1\in\Dom$ and thus $\tuple{w,w0},\tuple{w,w1}\in\interprets{\dot{R}}$.
                          Clearly, $\abs{w0}=\abs{w1}=i$ whence $w0,w1\in\interprets{L_i}$.
                          Furthermore, $(w0)_i=0$ whence $w0\in T_{\neg p_i}$;
                          likewise $(w1)_i=1$ and $w1\in T_{p_i}$.
                    \item (\ref{ltrue}): Let $w\in\interprets{L_i}\cap\interprets{T_{p_i}}$.
                          Then $\abs{w}=i$ and $w_i=1$ by definition.
                          Thus by agreement across precisifications, for any $Q\subseteq P$ we get $w\in(L_i\dland T_{p_i})^{\gamma(Q)}$, whence $w\in \bigcap_{Q\subseteq P} (L_i\dland T_{p_i})^{\gamma(Q)}$.
                    \item (\ref{lfalse}): Symmetric.
                    \item (\ref{sstart}): Let $w\in\interprets{L_k}$.
                          Then $\abs{w}=k$ and there is a $Q\subseteq P$ such that $w^Q=w$.
                          Since $w=w^Q\in\prefixes(w^Q)$ by definition, for $\gamma(Q)$ we thus have $w\in (\mathit{Select})^{\gamma(Q)}$.
                    \item (\ref{strue}): Let $\tuple{v,w}\in\interprets{\dot{R}}$ such that $w\in\interprets{T_{p_i}}\cap\interprets{\mathit{Select}}$.
                          Then $w\in\prefixes(w^Q)$, and either
                          (a) $\abs{w}=i$ and $w_i=1$, or
                          (b) $\abs{w}<i$ and $w^Q_i=1$.
                          By definition of $\interprets{\dot{R}}$ we have $v\in\prefixes(w)\subseteq\prefixes(w^Q)$, whence $v\in\interprets{\mathit{Select}}$.
                          In particular, $\abs{v}=i-1<i$ and in any case we have $w^Q_i=1$, thus $v\in\interprets{T_{p_i}}$.
                    \item (\ref{sfalse}): Symmetric.
                    \item (\ref{clause}): By definition.
                    \item (\ref{disjoint}): By contradiction:
                          Assume that there is a $Q\subseteq P$ such that for $\struct=\gamma(Q)$, there is some $w\in\interprets{T_{\clause_1}}\cap\ldots\cap\interprets{T_{\clause_n}}$.
                          Then by definition, for each $1\leq j\leq n$ there is an $\ell_j\in\clause_j$ such that $w\in\interprets{T_{\ell_j}}$.
                          Define $R_w = \set{ p\in P \guard w\in \interprets{T_{p}} } \cup \set{ \neg p \guard p\in P, w\in\interprets{T_{\neg p}}}$.
                          $R_w$ is consistent because for all $1\leq i\leq k$, we have $\interprets{T_{p_i}}\cap\interprets{T_{\neg p_i}}=\emptyset$.
                          We show $R_w\cap P\models\phi$ to obtain the desired contradiction with unsatisfiability of $\phi$.
                          Consider $\clause_j$.
                          We have $\ell_j\in\clause_j$ as above with $w\in\interprets{T_{\ell_j}}$, whence by definition $\ell_j\in R_w$.
                          Consequently, $R_w\cap P\models\ell_j$.
                          Since $\clause_j$ was chosen arbitrarily, we get $R_w\cap P\models\phi$.
                \end{itemize}
            \item[\normalfont``only if'':]
                Let $\phi$ be satisfiable.
                Then there is a $Q\subseteq P$ such that $Q\models\phi$.
                We show by contradiction that $\T_\phi$ is unsatisfiable.
                Assume that there is a Standpoint DL structure $\dlstruct=\tuple{\Dom,\Precs,\sigma,\gamma}$ such that $\dlstruct\models\T_\phi$.
                By $\dlstruct\models (\ref{lstart}) \land (\ref{lnext})$, in every $\pr\in\Precs$, $\dot{R}$ contains a full binary tree of depth $k$ where in each layer $i$, the nodes (individuals $\de_i\in\Dom$) are marked with $L_i$, and one of $T_{p_i}$ and $T_{\neg p_i}$, respectively.
                Due to the rigid role $\dot{R}$ being used and rigidity of $L_i\dland T_{(\neg)p_i}$ being enforced by (\ref{ltrue}) and (\ref{lfalse}), this part of the interpretation is “the same” across precisifications.
                Employing $\dlstruct\models (\ref{sstart})$, we now consider $\pr\in\Precs$ and the sequence
                $\de_0,\ldots,\de_k\in\Dom$ with $\de_0\in\interpretgp{L_0}$,
                $\tuple{\de_{i-1},\de_i}\in\interpretgp{\dot{R}}$ for all $1\leq i\leq k$,
                $\de_i\in\interpretgp{L_i}\cap\interpretgp{\mathit{Select}}$ for all $1\leq i\leq k$ such that for all $p_i\in P$:
                \begin{itemize}
                    \item $\de_i\in\interpretgp{T_{p_i}}$ whenever $p_i\in Q$,
                    \item $\de_i\in\interpretgp{T_{\neg p_i}}$ whenever $p_i\notin Q$.
                \end{itemize}
                Since $\dlstruct\models (\ref{lnext}) \land (\ref{strue}) \land (\ref{sfalse})$, it follows that for all $p\in P$:
                \begin{itemize}
                    \item $\de_1\in\interpretgp{T_{p}}$ whenever $p\in Q$,
                    \item $\de_1\in\interpretgp{T_{\neg p}}$ whenever $p\notin Q$.
                \end{itemize}
                Now since $Q\models\phi$, we get that $Q\models\clause_j$ for all $1\leq j\leq k$;
                that is, for every $\clause_j$ there is a literal $\ell_j\in\clause_j$ such that $Q\models\ell_j$.
                Now $Q\models\ell_j$ iff $\de_1\in\interpretgp{T_{\ell_j}}$ by the above.
                Thus, for every $\clause_j$ there is $\ell_j\in\clause_j$ such that $\de_1\in\interpretgp{T_{\ell_j}}$.
                Thus $\de_1\in T_{\clause_j}$ by $\dlstruct\models (\ref{clause})$.
                But then, since $\clause_j$ was chosen arbitrarily, we get $\de_1 \in \interpretgp{(T_{\clause_1}\dland\ldots\dland T_{\clause_n})}$ in contradiction to $\dlstruct\models (\ref{disjoint})$.
        \end{description}
    \end{proof}
\end{theorem}

\begin{definition}
    From a normalised Horn-$\mathcal{ALC}$ TBox $\mathcal{T}$, we obtain the target $\SELO$ TBox $\SELO(\mathcal{T})$ by
    \begin{itemize}[leftmargin=0.7cm]
        \item[(i)] declaring every original concept name as rigid via the axiom $A \sqsubseteq \standball A$ as well as
        \item[(ii)] replacing every axiom of the shape $A \sqsubseteq \exists R.B$ by the axiom
            \begin{linenomath*}
                $$A \sqsubseteq \standdall ((\exists \mathit{Src}.\{o\}) \sqcap (\exists R.(B \sqcap \exists \mathit{Tgt}.\{o\})))$$
            \end{linenomath*}
            (introducing two fresh role names $\mathit{Src}$ and $\mathit{Tgt}$), and replacing every axiom of the shape $A \sqsubseteq \forall r.B$ by the two axioms
            \begin{linenomath*}
                $$A \sqcap \exists R.\top \sqsubseteq (\exists \mathit{Src}.(\{o\} \sqcap \tilde{B})) \quad\text{and}\quad \exists \mathit{Tgt}.\tilde{B} \sqsubseteq B,$$
            \end{linenomath*}
            introducing a copy $\tilde{A}$ for every original concept name $A$.
    \end{itemize}
\end{definition}

\begin{theorem}
    Let $\mathcal{T}$ be a normalised Horn-$\mathcal{ALC}$ TBox. Then, $\mathcal{T}$ and $\SELO(\mathcal{T})$ are equisatisfiable.
\end{theorem}
\begin{proof}
    We show equisatisfiability of $\mathcal{T}$ and $\SELO(\mathcal{T})$ by providing constructions to obtain a model of $\mathcal{T}$ from a model of $\mathcal{T}'$ and vice versa.
    Let $\mathcal{I}=(\Dom,\cdot^\mathcal{I})$ be a model of $\mathcal{T}$. Then we construct a model
    $\dlstruct= \tuple{\Dom, \Precs, \sigma, \gamma}$ of $\SELO(\mathcal{T})$ as follows:
    \begin{itemize}
        \item $\Precs = \Roles \times \Dom \times \Dom$ with $\sigma(*) = \Precs$,
        \item pick one arbitrary but fixed $\delta_o \in \Dom$ and let $o^{\gamma(\pi)}=\delta_o$ for all $\pi \in \Precs$,
        \item $A^{\gamma(\pi)}=A^\mathcal{I}$ for all $\pi \in \Precs$, whereas
              $\tilde{A}^{\gamma((r,\delta_1,\delta_2))}= \{ \delta_o \mid \delta_2 \in A^\mathcal{I}\}$ for $A \in \Concepts$,
        \item $R^{\gamma((r,\delta_1,\delta_2))}=\{(\delta_1,\delta_2)\} \cap R^\mathcal{I}$, while
              $Src^{\gamma((r,\delta_1,\delta_2))}=\{(\delta_1,\delta_o)\}$ and
              $Tgt^{\gamma((r,\delta_1,\delta_2))}=\{(\delta_2,\delta_o)\}$.
    \end{itemize}

    \medskip

    For the other direction, let $\dlstruct= \tuple{\Dom, \Precs, \sigma, \gamma}$ be a model of $\SELO(\mathcal{T})$. Then we construct a model $\mathcal{I}=(\Dom,\cdot^\mathcal{I})$ of $\mathcal{T}$ as follows:
    \begin{itemize}
        \item $A^\mathcal{I} = A^{\gamma(\pi)}$ for any $\pi \in \Precs$ (the choice is irrelevant because all $A$ are rigid)
        \item $R^\mathcal{I} = \bigcup_{\pi \in \Precs}\{(\delta_1,\delta_2) \in R^{\gamma(\pi)} \mid (\delta_1,o^{\gamma(\pi)}) \in  Src^{\gamma(\pi)},\ (\delta_2,o^{\gamma(\pi)}) \in Tgt^{\gamma(\pi)}\}$
    \end{itemize}
\end{proof}

\end{document}
